# Supplementary material for: Online Heavy-tailed Change-point detection
Source: arXiv:2306.09548 source file (2023-07-03)
Supplement: Supplementary file 1 [file uai2023-supplement.tex]

\documentclass{uai2023} % for initial submission
% \documentclass[accepted]{uai2023} % after acceptance, for a revised
                                    % version; also before submission to
                                    % see how the non-anonymous paper
                                    % would look like

%% There is a class option to choose the math font
% \documentclass[mathfont=ptmx]{uai2023} % ptmx math instead of Computer
% Modern (has noticable issues)
% \documentclass[mathfont=newtx]{uai2023} % newtx fonts (improves upon
 % ptmx; less tested, no support)
% NOTE: Only keep *one* line above as appropriate, as it will be replaced
%       automatically for papers to be published. Do not make any other
%       change above this note for an accepted version.

%% Choose your variant of English; be consistent
\usepackage[american]{babel}
% \usepackage[british]{babel}

%% Some suggested packages, as needed:
\usepackage{natbib} % has a nice set of citation styles and commands
    \bibliographystyle{plainnat}
    
\usepackage{mathtools} % amsmath with fixes and additions
\usepackage{booktabs} % commands to create good-looking tables
\usepackage{tikz} % nice language for creating drawings and diagrams

% for cross referencing the main text
% PLEASE ONLY USE xr IN THE SUPPLEMENTARY MATERIAL. 
% In the main paper, hard code any cross-reference to the supplementary material. 
\usepackage{xr} 
\externaldocument{uai2023-template}

%% Provided macros
% \smaller: Because the class footnote size is essentially LaTeX's \small,
%           redefining \footnotesize, we provide the original \footnotesize
%           using this macro.
%           (Use only sparingly, e.g., in drawings, as it is quite small.)

%% Self-defined macros
 % just an example

\title{Title in Title Case\\(Supplementary Material)}

% The standard author block has changed for UAI 2023 to provide
% more space for long author lists and allow for complex affiliations
%
% All author information is authomatically removed by the class for the
% anonymous submission version of your paper, so you can already add your
% information below.
%
% Add authors
\author[1]{\href{mailto:<jj@example.edu>?Subject=Your UAI 2023 paper}{Jane~J.~von~O'L\'opez}{}}
\author[1]{Harry~Q.~Bovik}
\author[1,2]{Further~Coauthor}
\author[3]{Further~Coauthor}
\author[1]{Further~Coauthor}
\author[3]{Further~Coauthor}
\author[3,1]{Further~Coauthor}
% Add affiliations after the authors
\affil[1]{%
    Computer Science Dept.\\
    Cranberry University\\
    Pittsburgh, Pennsylvania, USA
}
\affil[2]{%
    Second Affiliation\\
    Address\\
    …
}
\affil[3]{%
    Another Affiliation\\
    Address\\
    …
  }
  
  \begin{document}
  
\onecolumn %% Turn this off if single column is desired for the supplement
\maketitle

This Supplementary Material should be submitted as a separate file. Please do not append the Supplementary Material to the main paper. 

Fig. \ref{fig:pitt} and Eq \ref{eq:example} in the main paper can be cross referenced using \texttt{xr}. 

\appendix
\section{Additional simulation results}
Table~\ref{tab:supp-data} lists additional simulation results; see also \citet{einstein} for a comparison. 

\begin{table}[!h]
    \centering
    \caption{An Interesting Table.} \label{tab:supp-data}
    \begin{tabular}{rl}
      \toprule % from booktabs package
      \bfseries Dataset & \bfseries Result\\
      \midrule % from booktabs package
      Data1 & 0.12345\\
      Data2 & 0.67890\\
      Data3 & 0.54321\\
      Data4 & 0.09876\\
      \bottomrule % from booktabs package
    \end{tabular}
\end{table}

\section{Math font exposition}
% NOTE: necessary when ptmx or no mathfont class option is given
\providecommand{\upGamma}{\Gamma}
\providecommand{\uppi}{\pi}
How math looks in equations is important:
\begin{equation*}
  F_{\alpha,\beta}^\eta(z) = \upGamma(\tfrac{3}{2}) \prod_{\ell=1}^\infty\eta \frac{z^\ell}{\ell} + \frac{1}{2\uppi}\int_{-\infty}^z\alpha \sum_{k=1}^\infty x^{\beta k}\mathrm{d}x.
\end{equation*}
However, one should not ignore how well math mixes with text:
The frobble function \(f\) transforms zabbies \(z\) into yannies \(y\).
It is a polynomial \(f(z)=\alpha z + \beta z^2\), where \(-n<\alpha<\beta/n\leq\gamma\), with \(\gamma\) a positive real number.

\bibliography{uai2023-template}

\end{document}
